# Supplementary material for: Latent Haldane Models
Source: arXiv:2411.08202 source file (2025-02-19)
Supplement: Supplementary file 1 [file generalizationPrincipleAppendix.pdf]

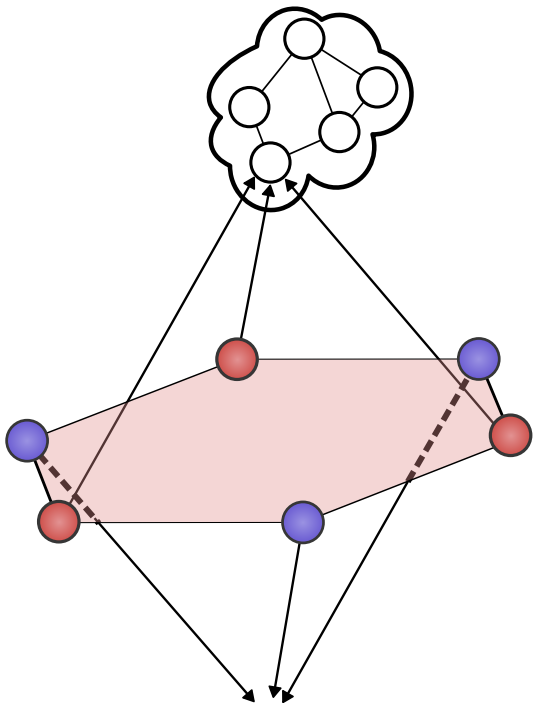

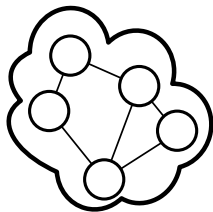

$$\tilde{t}$$

$$\tilde{t}e^{2\pi i/3}$$

$$\tilde{t}e^{4\pi i/3}$$

$$\tilde{t}e^{4\pi i/3}$$

$$\tilde{t}e^{2\pi i/3}$$

$$\tilde{t}$$
