# Supplementary material for: Latent Haldane Models
Source: arXiv:2411.08202 source file (2025-02-19)

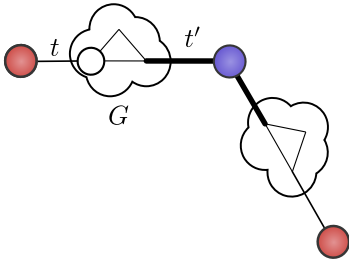

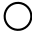

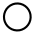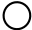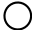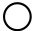

Supplement: Supplementary file 2 [file generalizationPrincipleSemenoffAppendix.pdf]
